# Supplementary material for: Bayesian analysis of ambulatory blood pressure dynamics with application to irregularly spaced sparse data
Source: arXiv:1511.05372 ancillary file (2017-01-10)

arXiv: arXiv:0001000

# SUPPLEMENTARY MATERIALS OF "BAYESIAN ANALYSIS OF AMBULATORY BLOOD PRESSURE DYNAMICS WITH APPLICATION TO IRREGULARLY SPACED SPARSE DATA"

By Zhao-Hua Lu*, Sy-Miin Chow†, Andrew Sherwood‡ and Hongtu Zhu*

*University of North Carolina at Chapel Hill*, Pennsylvania State University† and Duke University‡*

## S1. Details of the MCMC algorithms.

S1.1. *Posterior Computation.* Let $\mathbf{Y}_i = (\mathbf{y}_{i1}, \ldots, \mathbf{y}_{iT_i})$, $\mathbf{Y} = (\mathbf{Y}_1, \ldots, \mathbf{Y}_n)$, and $\boldsymbol{\theta} = \{\mathbf{b}, \boldsymbol{\mu}, \boldsymbol{\Lambda}, \boldsymbol{\Sigma}_{\boldsymbol{\epsilon}}\}$. Given the approximation in (3.4), we have

$$P_k(\mathbf{Y}, \mathbf{X}^{(k)}|\boldsymbol{\theta}) = P(\mathbf{Y}|\boldsymbol{\mu}, \boldsymbol{\Lambda}, \boldsymbol{\Sigma}_{\boldsymbol{\epsilon}}, \mathbf{X}^{(0)})P_k(\mathbf{X}^{(k)}|\mathbf{b})$$
$$= \prod_{i=1}^{n}\Big\{\prod_{j=1}^{T_i} P(\mathbf{y}_{ij}|\mathbf{x}_{ij}, \boldsymbol{\mu}, \boldsymbol{\Lambda}, \boldsymbol{\Sigma}_{\boldsymbol{\epsilon}}) \prod_{j=0}^{T_i^{(k)}-1} P_k(\mathbf{x}_{i,j+1}^{(k)}|\mathbf{x}_{ij}^{(k)}, \boldsymbol{\theta}_{xi})\Big\},$$

where

$$P(\mathbf{y}_{ij}|\mathbf{x}_{ij}, \boldsymbol{\mu}, \boldsymbol{\Lambda}, \boldsymbol{\Sigma}_{\boldsymbol{\epsilon}}) = \phi_p(\boldsymbol{\mu} + \boldsymbol{\Lambda}\mathbf{x}_{ij}, \boldsymbol{\Sigma}_{\boldsymbol{\epsilon}}). \quad \text{(S1.1)}$$

Let $y_{ijr}$ be the $r$th element of $\mathbf{y}_{ij}$, $\tilde{y}_{ijr} = y_{ijr} - \mu_r$, $\tilde{\mathbf{y}}_{ir} = (\tilde{y}_{i1r}, \ldots, \tilde{y}_{iT_ir})^T$, $\tilde{\mathbf{y}}_r = (\tilde{\mathbf{y}}_{1r}^T, \ldots, \tilde{\mathbf{y}}_{nr}^T)^T$, and $y_{ijr}^* = y_{ijr} - \boldsymbol{\Lambda}_r^T\mathbf{x}_{ij}$, for $1 \le j \le T_i$, $1 \le i \le n$. The Gibbs sampler cycles through the following steps:

1. Sample $\mu_r$ from $N(\mu_r^*, \sigma_{\mu r}^2)$, where $\mu_r^* = \sigma_{\mu r}^2(\sum_{i=1}^n \sum_{j=1}^{T_i} y_{ijr}^*/\sigma_{\epsilon r}^2 + \mu_{r0}/\sigma_{\mu 0}^2)$ and $\sigma_{\mu r}^2 = 1/(\sum_{i=1}^n T_i/\sigma_{\epsilon r}^2 + 1/\sigma_{\mu 0}^2)$;
2. Sample $\sigma_{\epsilon r}^2$ from $IG(a_{1r}+\sum_{i=1}^n T_i/2,\ a_{2r}^*)$ and then $\boldsymbol{\Lambda}_r$ from $N(\boldsymbol{\Lambda}_r^*,\ \sigma_{\epsilon r}^2\boldsymbol{\Sigma}_{\Lambda r}^*)$, where $a_{2r}^* = a_{2r} + (\tilde{\mathbf{y}}_r^T\tilde{\mathbf{y}}_r - \boldsymbol{\Lambda}_r^{*T}\boldsymbol{\Sigma}_{\Lambda r}^{*-1}\boldsymbol{\Lambda}_r^* + \boldsymbol{\Lambda}_{0r}^T\boldsymbol{\Sigma}_{\Lambda r}^{-1}\boldsymbol{\Lambda}_{0r}^T)/2$, in which $\boldsymbol{\Sigma}_{\Lambda r}^* = (\mathbf{X}^{(0)}\mathbf{X}^{(0)T} + \boldsymbol{\Sigma}_{\Lambda r}^{-1})^{-1}$ and $\boldsymbol{\Lambda}_r^* = \boldsymbol{\Sigma}_{\Lambda r}^*(\ \boldsymbol{\Sigma}_{\Lambda r}^{-1}\boldsymbol{\Lambda}_{0r} + \mathbf{X}^{(0)}\tilde{\mathbf{y}}_r)$;
3. Sample $\mathbf{b}$ from $P_k(\mathbf{b}|\mathbf{X}^{(k)}) \propto P_k(\mathbf{X}^{(k)}|\mathbf{b})P(\mathbf{b})$. More details are given in Supplement S1.5.
4. Sample $\mathbf{X}^{(k)}$ from $P_k(\mathbf{X}^{(k)}|\mathbf{Y}, \boldsymbol{\theta})$.

Samples are kept for posterior estimation and inference after the convergence of Gibbs sampler.

S1.2. *Multiresolution (MR) Algorithm.* Step 4 in the Gibbs sampler may be inefficient when $k$ is large. We develop an efficient multiresolution MCMC algorithm (Kou et al., 2012) to address such challenging issue, which consists of a global cross-resolution sampler and a Gibbs sampler that use two local samplers for Step 4: (i) a block updating scheme with $\tilde{k}+2$-step regularized Brownian bridge sampler (RBBS), and (ii) a Gibbs sampler that updates $\mathbf{x}_{ij}^{(k)}$ sequentially with 1-step RBBS. The MR algorithm is implemented as follows.

1. Construct $R$ resolutions $k_1 < k_2 < \ldots < k_R$ to be sequentially sampled from $k_1$ to $k_R$. The sequence of resolutions ranges from the lowest ($k_1$) to the highest ($k_R$) resolution and the differences between successive resolutions can follow any appropriately chosen scheme thought to help capture the global and local dynamics of the system. For instance, we may set $k_r^* = 2^{k_r}$ and $k_r = k_{r-1}+1$. In this way, $\mathbf{X}^{(k_r)}$ is constructed by augmenting $\mathbf{X}^{(k_{r-1})}$ with $\mathbf{x}_i(t)$ at the mid point between every $t_{i,j+1}^{(k_{r-1})}$ and $t_{ij}^{(k_{r-1})}$ for all $i$ and $j$. Let $\mathbf{X}^{(k_r)\backslash(k_{r-1})}$ be $\mathbf{x}_i(t)$ at the imputed mid points for all subjects, and $P_{k_r}$ be the posterior distribution at the $k_r-$th resolution for $r = 1, \ldots, R$.
2. Let $r = 1$. The $k_r$ missing data points are imputed between two observed time points in the Euler-Maruyama approximation. Monte Carlo samples from the posterior distribution $P_{k_r}(\boldsymbol{\theta}, \mathbf{X}^{(k_r)}|\mathbf{Y})$ are iteratively generated following the Gibbs sampler in Section S1.1. Two samplers described in Section 4.1.1 are used randomly with equal probability in Step 4 of the Gibbs sampler. After a sufficient burn-in period, an empirical posterior distribution is gathered as samples from $P_{k_r}(\boldsymbol{\theta}, \mathbf{X}^{(k_r)}|\mathbf{Y})$.
3. Proceed to the next higher resolution (i.e., let $r = r + 1$). Monte carlo samples from $P_{k_r}(\boldsymbol{\theta}, \mathbf{X}^{(k_r)}|\mathbf{Y})$ are generated by the Gibbs sampler similar to Step 2 and the cross-resolution sampler. In each iteration, a random number, $\alpha_1$, is generated from the uniform distribution on $[0, 1]$ to select the samplers:

    a. if $\alpha_1 < p_{\alpha 1}$, obtain samples from $P_{k_r}$ with the Gibbs sampler ($p_{\alpha 1} \in [0, 1]$ controls the proportion of the Gibbs sampler);

    b. else, sample $P_{k_r}$ with the cross-resolution global sampler in two steps. First, we sample the empirical samples $\boldsymbol{\theta}$ and $\mathbf{X}^{(k_{r-1})}$ from $P_{k_{r-1}}(\boldsymbol{\theta}, \mathbf{X}^{(k_{r-1})}|\mathbf{Y})$ uniformly. Then, $\mathbf{X}^{(k_r)\backslash(k_{r-1})}$ is obtained by generating $\mathbf{x}_i(t)$ at $(t_{i,j+1}^{(k_{r-1})} + t_{ij}^{(k_{r-1})})/2$ with the 1-step RBBS, leading to a complete new $\mathbf{X}^{(k_r)}$. The new sample of $(\boldsymbol{\theta}, \mathbf{X}^{(k_r)})$ is

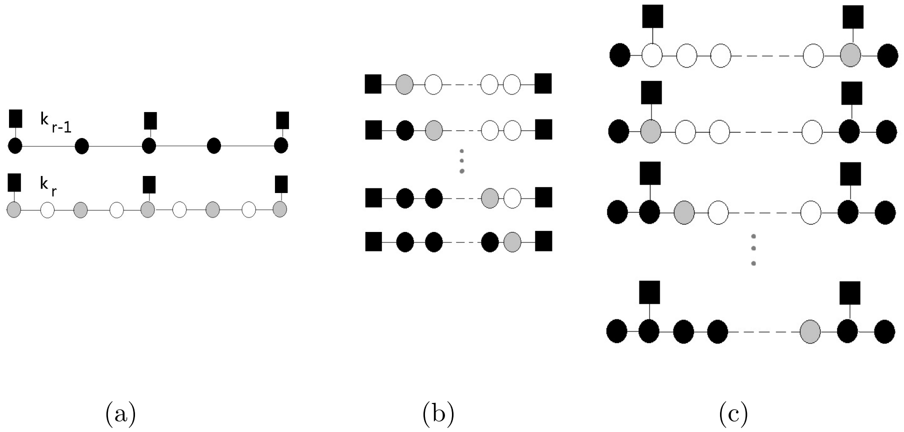


Fig S1: Graphical illustrations of (a) the cross-resolution sampler, (b) the $\tilde{k}$-step RBBS and (c) the $\tilde{k}+2$ step RBBS, respectively.

then accepted with a Metropolis-Hasting (MH)–type probability.

Iterate until a desired number of samples after burn-in. The retained samples form the posterior samples from $P_{k_r}(\boldsymbol{\theta}, \mathbf{X}^{(k_r)}|\mathbf{Y})$.

4. If $r < R$, return to step 3, otherwise exit the algorithm.

Block updating schemes (Durham and Gallant, 2002; Lindström, 2012) update highly correlated variables (in our case, $\mathbf{X}_{is}^{(k_r)} = (\mathbf{x}_{i,sk^*}^{(k_r)}, \ldots, \mathbf{x}_{i,(s+1)k^*}^{(k_r)})$) jointly to increase sampling efficiency. However, they are still local updating algorithms because $\mathbf{X}_{is}^{(k_r)}$ depends on $\mathbf{X}_{i,s-1}^{(k_r)}$ and $\mathbf{X}_{i,s+1}^{(k_r)}$. Their performances become worse for $\mathbf{X}_{is}^{(k_r)}$ strongly correlated with adjacent blocks, which may exist at small time intervals in irregularly spaced longitudinal data. Global updating samplers, which sample parameters and the stochastic processes simultaneously, may be used to further improve the MCMC performance. However, such samplers are often hard to construct due to the lack of efficient proposal distributions. One novel exception is the cross-resolution sampler in the MR algorithm.

S1.3. *Cross-resolution Sampler.* Cross-resolution sampler is a global sampler that updates all parameters and latent variables $(\mathbf{X}^{(k_r)}, \boldsymbol{\theta})$ jointly. It is essentially an independent MH sampler and does not depend the current state of $\mathbf{X}^{(k_r)}$ and $\boldsymbol{\theta}$. The target distribution is the posterior distribution in the $k_r$th resolution $P_{k_r}(\mathbf{X}^{(k_r)}, \boldsymbol{\theta}|\mathbf{Y})$. We break down $\mathbf{X}^{(k_r)}$ into $\mathbf{X}^{(k_{r-1})}$ and $\mathbf{X}^{(k_r)\backslash(k_{r-1})}$. The proposal sample $(\mathbf{X}^{(k_{r-1})*}, \boldsymbol{\theta}^*)$ is generated from the

empirical distribution of $P_{k_{r-1}}(\mathbf{X}^{(k_{r-1})}, \boldsymbol{\theta}|\mathbf{Y})$. Let $\boldsymbol{\mu}^*$, $\boldsymbol{\Lambda}^*$, $\boldsymbol{\Sigma_\epsilon}^*$ and $\mathbf{b}^*$ be the elements in $\boldsymbol{\theta}^*$, $\boldsymbol{\theta}_{xi}{}^* = g(\mathbf{w}_i, \mathbf{b}^*)$. $\mathbf{X}^{(k_r)\backslash(k_{r-1})*}$ is generated from

$$q^*_{k_r}(\mathbf{X}^{(k_r)\backslash(k_{r-1})}|\mathbf{X}^{(k_{r-1})*}, \mathbf{b}^*) = \prod_{i=1}^{n} \prod_{j=1}^{T_i^{(k_{r-1})}} q_1(\mathbf{x}^{(k_r)}_{i,2j-1}|\mathbf{x}^{(k_r)*}_{i,2j}, \mathbf{x}^{(k_r)*}_{i,2j-2}, \boldsymbol{\theta}_{xi}{}^*),$$

where $q_1(\mathbf{x}^{(k_r)}_{i,2j-1}|\mathbf{x}^{(k_r)*}_{i,2j}, \mathbf{x}^{(k_r)*}_{i,2j-2}, \boldsymbol{\theta}^*)$ is the proposal density of 1-step RBBS in equation (S1.4). The Metropolis-Hasting (MH)–type acceptance probability is:

$$\min\left[1, \frac{P_{k_r}(\mathbf{X}^{(k_r)*}, \boldsymbol{\theta}^*|\mathbf{Y})}{P_{k_r}(\mathbf{X}^{(k_r)}, \boldsymbol{\theta}|\mathbf{Y})} \frac{q^*_{k_r}(\mathbf{X}^{(k_r)\backslash(k_{r-1})}|\mathbf{X}^{(k_{r-1})}, \mathbf{b})P_{k_{r-1}}(\mathbf{X}^{(k_{r-1})}, \boldsymbol{\theta}|\mathbf{Y})}{q^*_{k_r}(\mathbf{X}^{(k_r)\backslash(k_{r-1})*}|\mathbf{X}^{(k_{r-1})*}, \mathbf{b}^*)P_{k_{r-1}}(\mathbf{X}^{(k_{r-1})*}, \boldsymbol{\theta}^*|\mathbf{Y})}\right].$$

Let $\mathbf{X}^{(0)*}$ be the submatrix of $\mathbf{X}^{(k_r)*}$ at observed time points. $\mathbf{X}^{(0)*}$ is included in $\mathbf{X}^{(k_1)*}$, and hence all $\mathbf{X}^{(k_r)*}$ for $r = 1, \ldots, R$. As a result, in the cross-resolution sampler, $\mathbf{X}^{(0)*}$ is always generated from $P_{k_{r-1}}(\mathbf{X}^{(k_{r-1})}, \boldsymbol{\theta}|\mathbf{Y})$ and is not generated from the $q^*_{k_r}(\mathbf{X}^{(k_r)\backslash(k_{r-1})}|\mathbf{X}^{(k_{r-1})*}, \mathbf{b}^*)$. Because

$$\begin{aligned}
&P_{k_r}(\mathbf{X}^{(k_r)}, \boldsymbol{\theta}|\mathbf{Y}) \propto P(\mathbf{Y}|\boldsymbol{\mu}, \boldsymbol{\Lambda}, \boldsymbol{\Sigma_\epsilon}, \mathbf{X}^{(0)})P_{k_r}(\mathbf{X}^{(k_r)}|\mathbf{b})P(\boldsymbol{\theta}),\\
&P_{k_{r-1}}(\mathbf{X}^{(k_{r-1})}, \boldsymbol{\theta}|\mathbf{Y}) \propto P(\mathbf{Y}|\boldsymbol{\mu}, \boldsymbol{\Lambda}, \boldsymbol{\Sigma_\epsilon}, \mathbf{X}^{(0)})P_{k_{r-1}}(\mathbf{X}^{(k_{r-1})}|\mathbf{b})P(\boldsymbol{\theta}),\\
&P_{k_r}(\mathbf{X}^{(k_r)*}, \boldsymbol{\theta}^*|\mathbf{Y}) \propto P(\mathbf{Y}|\boldsymbol{\mu}^*, \boldsymbol{\Lambda}^*, \boldsymbol{\Sigma_\epsilon}^*, \mathbf{X}^{(0)*})P_{k_r}(\mathbf{X}^{(k_r)*}|\mathbf{b}^*)P(\boldsymbol{\theta}^*),\\
&P_{k_{r-1}}(\mathbf{X}^{(k_{r-1})*}, \boldsymbol{\theta}^*|\mathbf{Y}) \propto P(\mathbf{Y}|\boldsymbol{\mu}^*, \boldsymbol{\Lambda}^*, \boldsymbol{\Sigma_\epsilon}^*, \mathbf{X}^{(0)*})P_{k_{r-1}}(\mathbf{X}^{(k_{r-1})*}|\mathbf{b}^*)P(\boldsymbol{\theta}^*),
\end{aligned}$$

$P(\mathbf{Y}|\boldsymbol{\mu}, \boldsymbol{\Lambda}, \boldsymbol{\Sigma_\epsilon}, \mathbf{X}^{(0)})$, $P(\mathbf{Y}|\boldsymbol{\mu}^*, \boldsymbol{\Lambda}^*, \boldsymbol{\Sigma_\epsilon}^*, \mathbf{X}^{(0)*})$, $P(\boldsymbol{\theta})$ and $P(\boldsymbol{\theta}^*)$ appear in both the numerator and the denominator, and are cancelled out in the acceptance probability:

$$\min\left[1, \frac{P_{k_r}(\mathbf{X}^{(k_r)^*}|\mathbf{b}^*)}{P_{k_r}(\mathbf{X}^{(k_r)}|\mathbf{b})} \frac{q^*_{k_r}(\mathbf{X}^{(k_r)\backslash(k_{r-1})}|\mathbf{X}^{(k_{r-1})}, \mathbf{b})P_{k_{r-1}}(\mathbf{X}^{(k_{r-1})}|\mathbf{b})}{q^*_{k_r}(\mathbf{X}^{(k_r)\backslash(k_{r-1})*}|\mathbf{X}^{(k_{r-1})*}, \mathbf{b}^*)P_{k_{r-1}}(\mathbf{X}^{(k_{r-1})*}|\mathbf{b}^*)}\right].$$

The cross-resolution sampler is essentially a MH sampler for the parameters $\boldsymbol{\theta}$ and latent processes at all time points $\mathbf{X}^{(k_r)}$ (including the observation times $\mathbf{X}^{(0)}$).

S1.4. *Local Updating Algorithms.* The superscripts $(k)$ of $\mathbf{x}$'s and $t$'s are suppressed for notational simplicity since the samplers are applied to different resolutions in the same manner. We use two local samplers for Step 4 of the Gibbs sampler in order to generate $\mathbf{X}$: (i) a 1-step RBBS that samples $\mathbf{x}_{ij}$ at each time point sequentially; and (ii) a block updating scheme

based on a $(\tilde{k}+2)$-step RBBS, which updates the latent variable scores in $\mathbf{X}_{is} = (\mathbf{x}_{i,sk^*}, \ldots, \mathbf{x}_{i,(s+1)k^*})$ jointly for $s = 0, \ldots, T_i - 1$. Analogues of samplers (i) and (ii) were proposed to sample univariate and multivariate nonlinear SDEs for a single subject, respectively, in Kou et al. (2012) and Lindström (2012). We will extend these samplers to handle latent SDEs for population data.

S1.4.1. *1-step RBBS.*. To implement the 1-step RBBS, different proposal distributions for the full conditional distributions of $\mathbf{x}_{ij}$ have to be used at the observed versus unobserved (i.e., imputed) time points. The full conditional distributions of the $\mathbf{x}_{ij}$ at the imputed (i.e., $(s-1)k^* < j < sk^*$) and observed time points (i.e., $j = sk^*$) for $s = 1, \ldots, T_i$ are given by

$$P(\mathbf{x}_{ij}|\mathbf{X}_{i,-j}, \boldsymbol{\theta}_{xi}) \propto P(\mathbf{x}_{i,j+1}|\mathbf{x}_{ij}, \boldsymbol{\theta}_{xi})P(\mathbf{x}_{ij}|\mathbf{x}_{i,j-1}, \boldsymbol{\theta}_{xi}), \tag{S1.2}$$

$$P(\mathbf{x}_{ij}|\mathbf{X}_{i,-j}, \boldsymbol{\theta}, \mathbf{Y}) \propto P(\mathbf{y}_{is}|\mathbf{x}_{ij}, \boldsymbol{\mu}, \boldsymbol{\Lambda}, \boldsymbol{\Sigma}_{\boldsymbol{\epsilon}})P(\mathbf{x}_{ij}|\mathbf{X}_{i,-j}, \boldsymbol{\theta}_{xi}), \tag{S1.3}$$

where the conditional distributions in the right-hand side are defined in (3.4) and (S1.1), and $\mathbf{X}_{i,-j}$ denotes the submatrix of $\mathbf{X}$ which includes all other $\mathbf{x}$'s except for $\mathbf{x}_{ij}$. As $\mathbf{x}_{ij}$ is involved in the nonlinear drift function in $P(\mathbf{x}_{i,j+1}|\mathbf{x}_{ij}, \boldsymbol{\theta}_{xi})$, (S1.2) and (S1.3) are nonstandard distributions of $\mathbf{x}_{ij}$. We use the 1-step RBBS with the following proposal distributions for (S1.2) and (S1.3), respectively:

$$\begin{aligned} & q_1(\mathbf{x}_{ij}|\mathbf{x}_{i,j+1}, \mathbf{x}_{i,j-1}, \boldsymbol{\theta}_{xi}) \\ \propto\ & P^*(\mathbf{x}_{i,j+1}|\mathbf{x}_{ij}, \mathbf{x}_{i,j-1}, \boldsymbol{\theta}_{xi})P(\mathbf{x}_{ij}|\mathbf{x}_{i,j-1}, \boldsymbol{\theta}_{xi}), \end{aligned} \tag{S1.4}$$

$$\begin{aligned} & q_2(\mathbf{x}_{ij}|\mathbf{x}_{i,j+1}, \mathbf{x}_{i,j-1}, \mathbf{y}_{is}, \boldsymbol{\theta}) \\ \propto\ & P(\mathbf{y}_{is}|\mathbf{x}_{ij}, \boldsymbol{\mu}, \boldsymbol{\Lambda}, \boldsymbol{\Sigma}_{\boldsymbol{\epsilon}})q_1(\mathbf{x}_{ij}|\mathbf{x}_{i,j+1}, \mathbf{x}_{i,j-1}, \boldsymbol{\theta}_{xi}), \end{aligned} \tag{S1.5}$$

where $P^*(\mathbf{x}_{i,j+1}|\mathbf{x}_{ij}, \mathbf{x}_{i,j-1}, \boldsymbol{\theta}_{xi})$ is given by

$$\phi_q\left(\mathbf{x}_{ij} + \mathbf{f}(\mathbf{x}_{i,j-1}, \boldsymbol{\theta}_{xi})\Delta t_{ij},\ \boldsymbol{\Sigma}(\mathbf{x}_{i,j-1}, \boldsymbol{\theta}_{xi})\big[(t_{i,j+1} - t_{ij}) + \alpha\frac{(t_{i,j+1} - t_{ij})^2}{(t_{ij} - t_{i,j-1})}\big]\right),$$

in which $\alpha$ is a fixed scalar in $[0.01, 1]$. Moreover, $\alpha = 0.2$ is used through out the paper, which is in the range suggested by Lindström (2012). The $\alpha(t_{i,j+1} - t_{ij})^2/(t_{ij} - t_{i,j-1})$ was proposed by Lindström (2012) to correct the approximation bias induced by $P^*$, which was shown to be critical for capturing the nonlinear drifts of processes observed at sparse time points when the model is dominated by the nonlinear drift functions. Otherwise, the linear bridge (e.g., Durham and Gallant, 2002) may be used, which is equivalent to setting $\alpha = 0$. The densities in (S1.4) and (S1.5) are multivariate Gaussian densities of $\mathbf{x}_{ij}$. Denote $C_{tij} = \Delta t^*_{ij}\Delta t_{i,j-1}/(\Delta t^*_{ij} + \Delta t_{i,j-1})$,

and $\Delta t_{ij}^* = \{(t_{i,j+1} - t_{ij}) + \alpha(t_{i,j+1} - t_{ij})^2/(t_{ij} - t_{i,j-1})\}$. $q_1(\cdot|\cdot)$ in (S1.4) is a $q$-dimensional multivariate Gaussian density with mean and covariance matrix

$$\begin{aligned}\boldsymbol{\Sigma}_{2\mathbf{x}_{ij}} &= C_{tij}\boldsymbol{\Sigma}(\mathbf{x}_{i,j-1}, \boldsymbol{\theta}_{xi}),\\ \boldsymbol{\mu}_{2\mathbf{x}_{ij}} &= C_{tij}\left(\frac{\mathbf{x}_{i,j+1} - \Delta t_{ij}\mathbf{f}(\mathbf{x}_{i,j-1}, \boldsymbol{\theta}_{xi})}{\Delta t_{ij}^*} + \frac{\mathbf{x}_{i,j-1} + \Delta t_{i,j-1}\mathbf{f}(\mathbf{x}_{i,j-1}, \boldsymbol{\theta}_{xi})}{\Delta t_{i,j-1}}\right).\end{aligned}$$

$q_2(\cdot|\cdot)$ in (S1.5) is a $q$-dimensional multivariate Gaussian density with mean and covariance matrix

$$\text{(S1.6)} \qquad \begin{aligned}\boldsymbol{\Sigma}^*_{2\mathbf{x}_{ij}} &= \left[\boldsymbol{\Sigma}^{-1}_{2\mathbf{x}_{ij}} + \boldsymbol{\Lambda}^T\boldsymbol{\Sigma}_{\boldsymbol{\epsilon}}{}^{-1}\boldsymbol{\Lambda}\right]^{-1}, \quad \text{and}\\ \boldsymbol{\mu}^*_{2\mathbf{x}_{ij}} &= \boldsymbol{\Sigma}^*_{2\mathbf{x}_{ij}}\left[\boldsymbol{\Sigma}^{-1}_{2\mathbf{x}_{ij}}\boldsymbol{\mu}_{2\mathbf{x}_{ij}} + \boldsymbol{\Lambda}^T\boldsymbol{\Sigma}_{\boldsymbol{\epsilon}}{}^{-1}(\mathbf{y}_{is} - \boldsymbol{\mu})\right].\end{aligned}$$

The MH acceptance probability for a proposal sample $\mathbf{x}_{ij}^*$ generated from $q_1(\cdot|\cdot)$ and $q_2(\cdot|\cdot)$ is given by

$$\min\left\{1, \frac{P(\mathbf{x}_{i,j+1}|\mathbf{x}_{ij}^*, \boldsymbol{\theta}_{xi})P^*(\mathbf{x}_{i,j+1}|\mathbf{x}_{ij}, \mathbf{x}_{i,j-1}, \boldsymbol{\theta}_{xi})}{P(\mathbf{x}_{i,j+1}|\mathbf{x}_{ij}, \boldsymbol{\theta}_{xi})P^*(\mathbf{x}_{i,j+1}|\mathbf{x}_{ij}^*, \mathbf{x}_{i,j-1}, \boldsymbol{\theta}_{xi})}\right\}.$$

The acceptance rate is close to 1 if $\Delta t_{ij}$ is small because $\mathbf{f}(\mathbf{x}_{i,j-1}, \boldsymbol{\theta}_{xi})$ and $\boldsymbol{\Sigma}(\mathbf{x}_{i,j-1}, \boldsymbol{\theta}_{xi})$ are close to $\mathbf{f}(\mathbf{x}_{ij}, \boldsymbol{\theta}_{xi})$ and $\boldsymbol{\Sigma}(\mathbf{x}_{ij}, \boldsymbol{\theta}_{xi})$, respectively.

S1.4.2. *($\tilde{k}$+2)-step RBBS.* Let $\tilde{k} = k^* - 1$. As $k$ gets larger, sampling each $\mathbf{x}_{ij}$ sequentially becomes progressively less efficient because of the strong correlations among the $\mathbf{x}_{ij}$'s. When $\mathbf{x}_{i,sk^*}$ and $\mathbf{x}_{i,(s+1)k^*}$ are observed, Lindström (2012) proposed to sample $\tilde{\mathbf{X}}_{is} = (\mathbf{x}_{i,sk^*+1}, \ldots, \mathbf{x}_{i,(s+1)k^*-1})$ as a whole block for $s = 0, \ldots, T_i - 1$. Figure S1b illustrates the procedure of this block sampler. Squares represent observed time points and circles stand for imputed time points. The circles are generated sequentially in $k$ steps. Grey circles represent the time point, where the processes are being generated, black circles represent time points being conditional on at the current stage, and white circles are time points not considered in this stage. Essentially, this sampler utilizes the 1-step RBBS $\tilde{k}$ times. The proposal distribution is

$$\text{(S1.7)} \quad q_L(\tilde{\mathbf{X}}_{is}|\mathbf{x}_{i,sk^*}, \mathbf{x}_{i,(s+1)k^*}, \boldsymbol{\theta}_{xi}) = \prod_{j=sk^*+1}^{sk^*+k} q_1(\mathbf{x}_{ij}|\mathbf{x}_{i,(s+1)k^*}, \mathbf{x}_{i,j-1}, \boldsymbol{\theta}_{xi}),$$

which is a sequential implementation of $\tilde{k}$-step RBBS for $\mathbf{x}_{i,sk^*+1}, \ldots, \mathbf{x}_{i,sk^*+k}$. To account that $\mathbf{x}_{i,sk^*}$ and $\mathbf{x}_{i,(s+1)k^*}$ are unobserved, we propose a new

$(\tilde{k}+2)$-step RBBS for generating $\mathbf{X}_{is} = (\mathbf{x}_{i,sk^*}, \ldots, \mathbf{x}_{i,(s+1)k^*})$ from

$$\begin{aligned}(S1.8)\quad & q_B(\mathbf{X}_{is}|\mathbf{x}_{i,sk^*-1}, \mathbf{x}_{i,(s+1)k^*+1}, \mathbf{y}_{is}, \mathbf{y}_{i,s+1}, \boldsymbol{\theta}) \\ =& q_2(\mathbf{x}_{i,(s+1)k^*}|\mathbf{x}_{i,sk^*-1}, \mathbf{x}_{i,(s+1)k^*+1}, \mathbf{y}_{i,s+1}, \boldsymbol{\theta})\times \\ & q_2(\mathbf{x}_{i,sk^*}|\mathbf{x}_{i,(s+1)k^*}, \mathbf{x}_{i,sk^*-1}, \mathbf{y}_{is}, \boldsymbol{\theta}) q_L(\tilde{\mathbf{X}}_{is}|\mathbf{x}_{i,sk^*}, \mathbf{x}_{i,(s+1)k^*}, \boldsymbol{\theta}_{xi}).\end{aligned}$$

More specifically, elements of the proposal sample $\mathbf{X}^*_{is} = (\mathbf{x}^*_{i,sk^*}, \ldots, \mathbf{x}^*_{i,(s+1)k^*})$ are sequentially generated as follows:

- generate $\mathbf{x}^*_{i,(s+1)k^*}$ from $q_2(\mathbf{x}_{i,(s+1)k^*}|\mathbf{x}_{i,sk^*-1}, \mathbf{x}_{i,(s+1)k^*+1}, \mathbf{y}_{i,s+1}, \boldsymbol{\theta})$;
- generate $\mathbf{x}^*_{i,sk^*}$ from $q_2(\mathbf{x}_{i,sk^*}|\mathbf{x}^*_{i,(s+1)k^*}, \mathbf{x}_{i,sk^*-1}, \mathbf{y}_{is}, \boldsymbol{\theta})$;
- generate $\mathbf{x}_{ij}$ from $q_1(\mathbf{x}_{ij}|\mathbf{x}^*_{i,(s+1)k^*}, \mathbf{x}^*_{i,j-1}, \boldsymbol{\theta}_{xi})$, $j = sk^*+1, \ldots, sk^*+k$.

The target distribution

$$\begin{aligned} & P(\mathbf{X}^*_{is}|\mathbf{x}_{i,(s+1)k^*+1}, \mathbf{x}_{i,sk^*-1}, \mathbf{y}_{is}, \mathbf{y}_{i,s+1}, \boldsymbol{\theta}) \\ \propto\ & P(\mathbf{y}_{is}, \mathbf{y}_{i,s+1}, \mathbf{X}^*_{is}|\mathbf{x}_{i,(s+1)k^*+1}, \mathbf{x}_{i,sk^*-1}, \boldsymbol{\theta}) \\ =\ & P(\mathbf{y}_{is}|\mathbf{x}^*_{i,sk^*}, \boldsymbol{\mu}, \boldsymbol{\Lambda}, \boldsymbol{\Sigma}_{\boldsymbol{\epsilon}}) P(\mathbf{y}_{i,s+1}|\mathbf{x}^*_{i,(s+1)k^*}, \boldsymbol{\mu}, \boldsymbol{\Lambda}, \boldsymbol{\Sigma}_{\boldsymbol{\epsilon}}) \times \\ & P(\mathbf{X}^*_{is}|\mathbf{x}_{i,(s+1)k^*+1}, \mathbf{x}_{i,sk^*-1}, \boldsymbol{\theta}_{xi}),\end{aligned}$$

where $P(\mathbf{X}^*_{is}|\mathbf{x}_{i,(s+1)k^*+1}, \mathbf{x}_{i,sk^*-1}, \boldsymbol{\theta}_{xi})$ is

$$P(\mathbf{x}^*_{i,sk^*}|\mathbf{x}_{i,sk^*-1}, \boldsymbol{\theta}_{xi}) \Bigg\{ \prod_{j=sk^*}^{(s+1)k^*-1} P(\mathbf{x}^*_{i,j+1}|\mathbf{x}^*_{ij}, \boldsymbol{\theta}_{xi}) \Bigg\} P(\mathbf{x}_{i,(s+1)k^*+1}|\mathbf{x}^*_{i,(s+1)k^*}, \boldsymbol{\theta}_{xi}).$$

The proposal distribution $q_B(\mathbf{X}^*_{is}|\mathbf{x}_{i,sk^*-1}, \mathbf{x}_{i,(s+1)k^*+1}, \mathbf{y}_{is}, \mathbf{y}_{i,s+1}, \boldsymbol{\theta})$ is

$$\begin{aligned} & q_2(\mathbf{x}^*_{i,(s+1)k^*}|\mathbf{x}_{i,sk^*-1}, \mathbf{x}_{i,(s+1)k^*+1}, \mathbf{y}_{i,s+1}, \boldsymbol{\theta})\times \\ & q_2(\mathbf{x}^*_{i,sk^*}|\mathbf{x}^*_{i,(s+1)k^*}, \mathbf{x}_{i,sk^*-1}, \mathbf{y}_{is}, \boldsymbol{\theta})\times \\ & q_L(\tilde{\mathbf{X}}^*_{is}|\mathbf{x}^*_{i,sk^*}, \mathbf{x}^*_{i,(s+1)k^*}, \boldsymbol{\theta}_{xi}).\end{aligned}$$

Let $q_B^-(\mathbf{X}^*_{is}|\mathbf{x}_{i,sk^*-1}, \mathbf{x}_{i,(s+1)k^*+1}, \boldsymbol{\theta}_{xi})$ be

$$\begin{aligned} & q_1(\mathbf{x}^*_{i,(s+1)k^*}|\mathbf{x}_{i,sk^*-1}, \mathbf{x}_{i,(s+1)k^*+1}, \boldsymbol{\theta}_{xi}) q_1(\mathbf{x}^*_{i,sk^*}|\mathbf{x}^*_{i,(s+1)k^*}, \mathbf{x}_{i,sk^*-1}, \boldsymbol{\theta}_{xi}) \\ & q_L(\tilde{\mathbf{X}}^*_{is}|\mathbf{x}^*_{i,sk^*}, \mathbf{x}^*_{i,(s+1)k^*}, \boldsymbol{\theta}_{xi}).\end{aligned}$$

The MH acceptance probability for $\mathbf{X}^*_{is}$ is given by

$$\min\left\{1, \frac{P(\mathbf{X}^*_{is}|\mathbf{x}_{i,(s+1)k^*+1}, \mathbf{x}_{i,sk^*-1}, \boldsymbol{\theta}_{xi}) q_B^-(\mathbf{X}_{is}|\mathbf{x}_{i,sk^*-1}, \mathbf{x}_{i,(s+1)k^*+1}, \boldsymbol{\theta}_{xi})}{P(\mathbf{X}_{is}|\mathbf{x}_{i,(s+1)k^*+1}, \mathbf{x}_{i,sk^*-1}, \boldsymbol{\theta}_{xi}) q_B^-(\mathbf{X}^*_{is}|\mathbf{x}_{i,sk^*-1}, \mathbf{x}_{i,(s+1)k^*+1}, \boldsymbol{\theta}_{xi})}\right\}.$$

$P(\mathbf{y}_{is}|\mathbf{x}_{i,sk^*}, \boldsymbol{\mu}, \boldsymbol{\Lambda}, \boldsymbol{\Sigma}_{\boldsymbol{\epsilon}})$, $P(\mathbf{y}_{i,s+1}|\mathbf{x}_{i,(s+1)k^*}, \boldsymbol{\mu}, \boldsymbol{\Lambda}, \boldsymbol{\Sigma}_{\boldsymbol{\epsilon}})$, $P(\mathbf{y}_{is}|\mathbf{x}^*_{i,sk^*}, \boldsymbol{\mu}, \boldsymbol{\Lambda}, \boldsymbol{\Sigma}_{\boldsymbol{\epsilon}})$ and $P(\mathbf{y}_{i,s+1}|\mathbf{x}^*_{i,(s+1)k^*}, \boldsymbol{\mu}, \boldsymbol{\Lambda}, \boldsymbol{\Sigma}_{\boldsymbol{\epsilon}})$ are cancelled out because they appear in both the numerator and the denominator.

Different orders of $\mathbf{x}$ in $q_2(\cdot|\cdot)$ define different conditional distributions. The order in $q_2(\mathbf{x}^*_{i,(s+1)k^*}|\mathbf{x}_{i,sk^*-1}, \mathbf{x}_{i,(s+1)k^*+1}, \mathbf{y}_{i,s+1}, \boldsymbol{\theta})$ is time reversed because $P^*$ in (S1.5) is used to account for the bias caused by the larger time interval between $\mathbf{x}_{i,sk^*-1}$ and $\mathbf{x}_{i,(s+1)k^*}$.

As shown in (Lindström, 2012), the tuning parameter is the size of the squared truncation bias compared to the conditional variance under Euler-Maruyama approximation, which is hard to estimate because it depends on the state of the (latent) processes and the unknown parameters. To empirically select a tuning parameter, we run a few short MCMC chains with different tuning parameters and select the one that produces the most efficient MCMC samples.

Golightly and Wilkinson (2008) also developed an alternative block updating algorithm for sampling overlapping blocks $(\mathbf{x}_{i,sk^*+1}, \ldots, \mathbf{x}_{i,(s+2)k^*-1})$ with $2\tilde{k}+1$ time points. The model they considered consists of multivariate stochastic processes with partial and discrete observations. More specifically, certain elements in $\mathbf{x}_{ij}$ are observed directly and others are observed with errors. The algorithm is efficient in this setting because it is a global updating algorithm. Compared to the $(\tilde{k}+2)-$th block in (S1.8), one advantage of the $(2\tilde{k}+1)-$th block is that information from $\mathbf{x}_{i,sk^*}$, $\mathbf{x}_{i,(s+1)k^*}$, and $\mathbf{x}_{i,(s+2)k^*}$ that are at least partially observed is used. In contrast, only $\mathbf{x}_{i,sk^*}$, $\mathbf{x}_{i,(s+1)k^*}$ are used by the $\tilde{k}+2$ step RBBS. In our model, $\mathbf{x}_{ij}$ is fully latent. The full conditional distribution of the $(2\tilde{k}+1)-$th block depends on $\mathbf{x}_{i,sk^*}$, $\mathbf{y}_{i,s+1}$ and $\mathbf{x}_{i,(s+2)k^*}$. In comparison, that of the $(\tilde{k}+2)-$th block is conditional on $\mathbf{x}_{i,sk^*-1}$, $\mathbf{y}_{is}$, $\mathbf{y}_{i,s+1}$ and $\mathbf{x}_{i,(s+1)k^*+1}$. The additional information from $\mathbf{y}_{is}$ may be helpful to increase the convergence of the MCMC algorithm. We use the $(\tilde{k}+2)$ block updating algorithm in our study.

S1.5. *Sampling Parameters in SDEs.* In the dual OU model, we set $\mathbf{b} = (\boldsymbol{\beta}_1^T, \ldots, \boldsymbol{\beta}_6^T, \psi)^T$. The full conditional distribution of $\psi$ is an inverse Gamma distribution. The derivation and sampling are standard. The $\boldsymbol{\beta}_j$s are sampled with Metropolis-Hastings algorithm from their full conditional distributions proportional to $P_k(\mathbf{X}^{(k)}|\mathbf{b})p(\boldsymbol{\beta}_j)$. The proposal distributions are constructed with the hit-and-run Metropolis sampler (Chen and Schmeiser, 1993), which is convenient for parameters in truncated spaces (e.g., $\boldsymbol{\beta}_1$).

**S2. Additional Analysis of the Case Study.** To compare the MR algorithm with local algorithms, we reanalyzed the same dataset using only

Steps 1 and 2 in the MR algorithm with the 4th resolution, which is essentially a Gibbs sampler with only one resolution (termed "**Local algorithm 1+2**"). To further investigate the efficiency of the block updating scheme based on $(\tilde{k}+2)$-step RBBS over the 1-step RBBS, we applied the Gibbs sampler, Step 4 of which only consists of 1-step RBBS (termed "**Local algorithm 1**"). The MR algorithm improves the efficiency of the MCMC algorithm by dramatically reducing the autocorrelations of the MCMC samples of most parameters. Figure S2 shows the autocorrelation plots of MCMC samples of $\beta_{11}$, $\beta_{61}$, and $\psi$, and trajectories of MCMC samples of $\psi$ generated by the local algorithm 1, 1+2, and the MR algorithm, respectively. The local algorithms produce inaccurate estimates and SEs of some coefficients based on inefficient MCMC samples. For example, the Est and SE of $\beta_{61}$ based on the local algorithm 1 are 1.278 and 0.577, leading to invalid inference results.

## REFERENCES

Chen, M.-H. and Schmeiser, B. (1993). Performance of the Gibbs, hit-and-run, and Metropolis samplers. *Journal of computational and graphical statistics* **2** 251–272.

Durham, G. B. and Gallant, A. R. (2002). Numerical techniques for maximum likelihood estimation of continuous-time diffusion processes. *Journal of Business & Economic Statistics* **20** 297-316.

Golightly, A. and Wilkinson, D. J. (2008). Bayesian inference for nonlinear multivariate diffusion models observed with error. *Computational Statistics & Data Analysis* **52** 1674 - 1693.

Kou, S. C., Olding, B. P., Lysy, M. and Liu, J. S. (2012). A multiresolution method for parameter estimation of diffusion processes. *Journal of the American Statistical Association* **107** 1558–1574.

Lindström, E. (2012). A regularized bridge sampler for sparsely sampled diffusions. *Statistics and Computing* **22** 615-623. 10.1007/s11222-011-9255-y.

Department of Biostatistics,
University of North Carolina at Chapel Hill
Chapel Hill, NC 27599, USA
E-mail: luz@email.unc.edu
htzhu@email.unc.edu

Dept. of Human Development and Family Studies
Penn State University
118 Henderson South Building
University Park, PA 16803
E-mail: quc16@psu.edu

Psychology and Neuroscience
4569 Hosp South
Campus Box 3119 Med Ctr
E-mail: andrew.sherwood@duke.edu

Fig S2: Panels (a)-(c) are the autocorrelations of the MCMC samples of $\beta_{11}$, $\beta_{62}$ and $\psi$. Red triangles, black circles, and blue crosses are the autocorrelations of MCMC samples by the local algorithms 1, 1+2, and the MR algorithm, respectively. Panels (d)-(f) are the trajectories of MCMC samples of $\psi$ produced by the local sampler 1, 1+2, and the MR algorith, respectively.

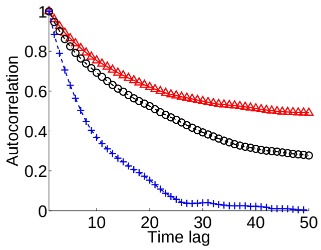


(a)

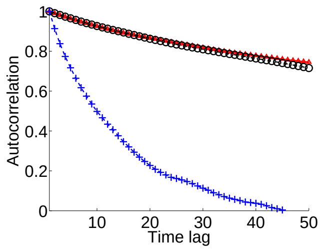


(b)

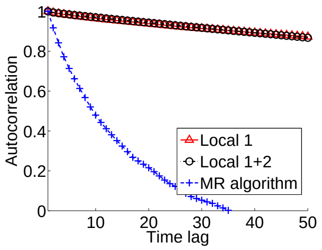


(c)

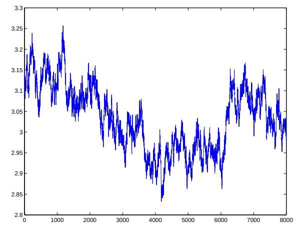

(d)

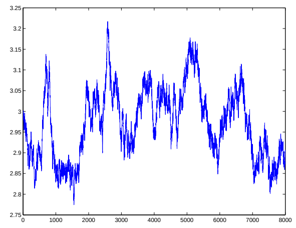

(e)

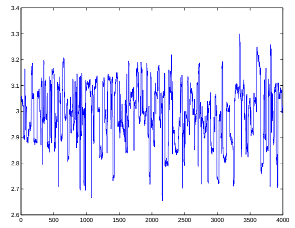

(f)

Fig S3: Observed and predicted trajectories of 3 randomly selected subjects in the case study. Each row is for a subject. From left to right are the trajectories of SBP, DBP, HR, respectively. Black solid curves are the observed trajectories. Curves with red crosses are the estimated posterior median. Curves with blue circles are the 95% pointwise credible intervals.

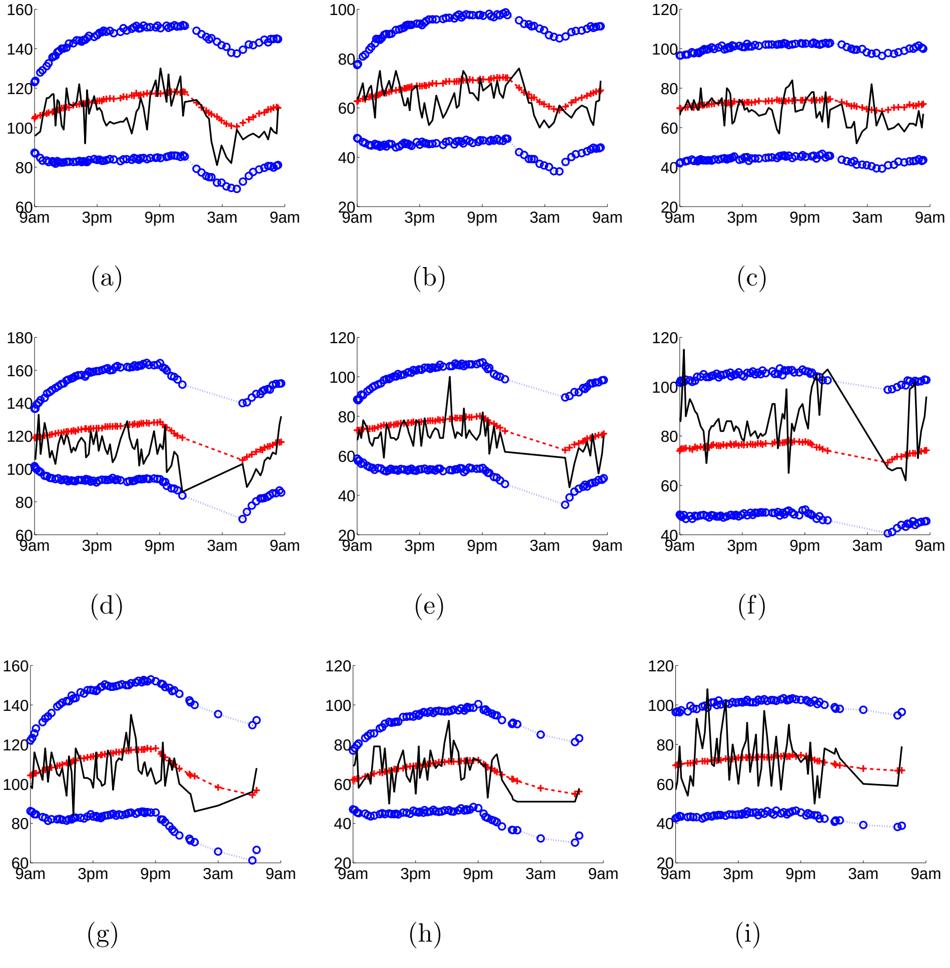

Supplement: Supplementary file 1 [file AOAS846_supp.pdf]
